# Supplementary material for: SUFFICIENT: A scan-specific unsupervised deep learning framework for high-resolution 3D isotropic fetal brain MRI reconstruction
Source: arXiv:2505.17472 source file (2025-05-26)
Supplement: Supplementary file 1 [file appendix.tex]

\appendices
\section*{Appendix}
\subsection{Gaussian Mixture Models (GMMs) Analysis}

The study detailed in \cite{laidlaw1998partial} has established that voxel intensities from pure tissue adhere to a Gaussian distribution. In accordance with this, we utilize a Gaussian Mixture Model (GMM) with three components to characterize voxel intensity distribution in an image. Fig. \ref{gmm} illustrates GMMs and their three components for five different methods applied to clinical data. Cyan bars depict voxel intensity distribution in a selected image region containing gray matter (GM), white matter (WM), and cerebrospinal fluid (CSF). The GMM with three components, fitted to the voxel intensity distribution, is shown by the solid line, while dashed lines represent GMM components corresponding to WM, GM, and CSF. Notably, Fig. \ref{gmm} highlights the distinctiveness of the three components of SUFFICIENT among GMMs from five baseline methods. To assess the partial volume effect (PVE), we implemented a threshold-based approach \cite{sui2022scan}. Voxels were classified into the k-th tissue (GM/WM/CSF) if their intensities fell within $\pm \delta_k$ of the mean of the k-th Gaussian component, where $\delta_k$ represents the corresponding half full width at half maximum (FWHM). This method measures the percentage of voxels outside these ranges, serving as a proxy for PVE, with narrower components having a higher probability of generating PVE. The broader Gaussian component exhibited by SUFFICIENT indicates a smaller PVE.

\begin{figure}[htbp]
    \centerline{\includegraphics[width=\columnwidth]{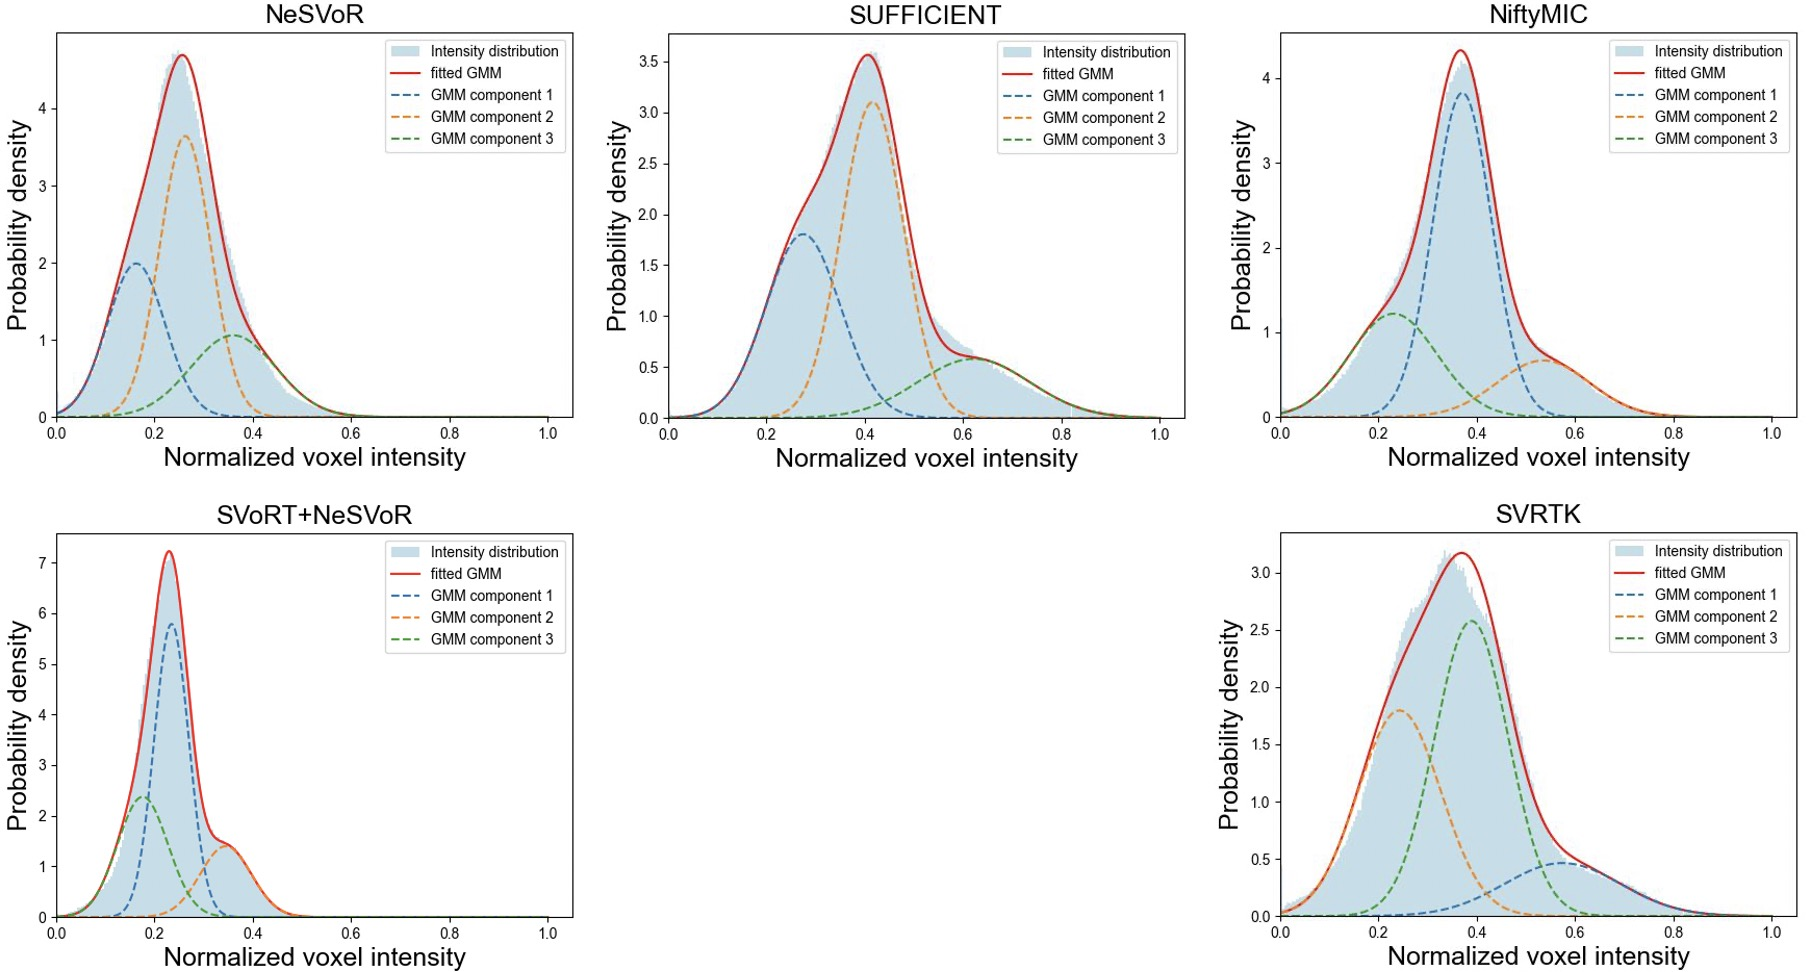}}
    \caption{Distribution of voxel intensities from a selected clinical image region containing CSF, GM, and WM, fitted with a three-component Gaussian mixture model (GMM). The distinct components represent WM, GM, and CSF, from left to right, respectively. } 
    
    \label{gmm}
    % \vspace{-0.2in}
    \end{figure}
    
    \begin{figure}[htbp]
    \centerline{\includegraphics[width=\columnwidth]{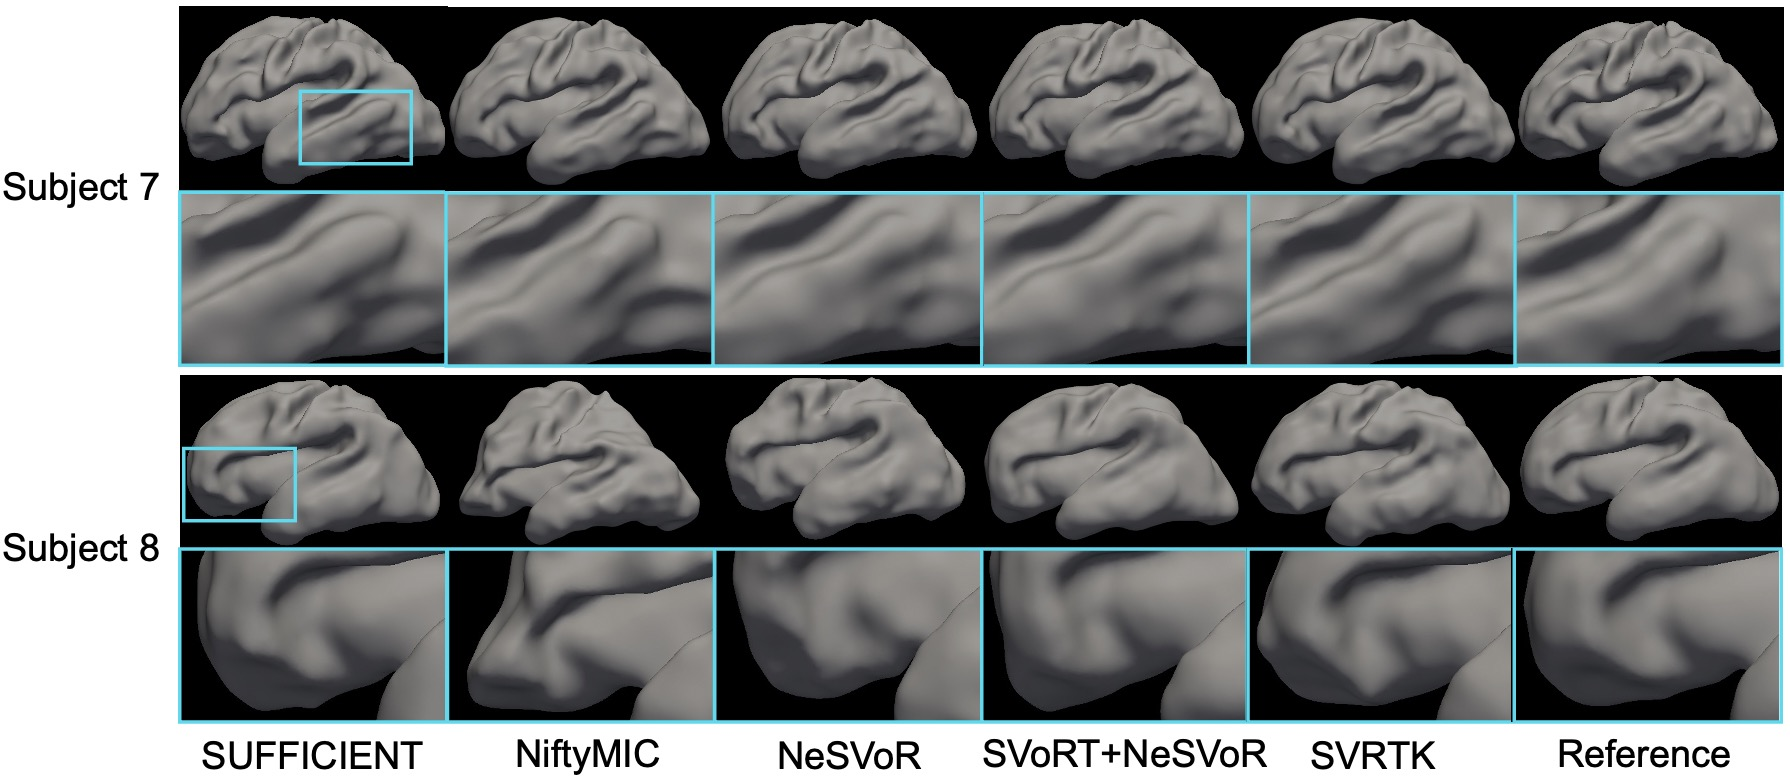}}
    \caption{Qualitative comparison of 3D fetal brain cortical surfaces constructed from the volumes reconstructed by five reconstruction methods on two fetal brain subjects. For reference, the cortical surfaces from an atlas matched to the corresponding gestational age are also included. } 
    
    \label{surface}
    % \vspace{-0.2in}
    \end{figure}

\subsection{The 3D cortical surface of the clinical dataset}

    Fig. \ref{surface} visually presents the 3D fetal brain cortical surfaces generated from volumes reconstructed by five methods. Notably, the 3D cortical surfaces of volumes produced by SUFFICIENT exhibit superior results, particularly in terms of cortex continuity. This is evident in the zoomed-in image of the blue box, where the 3D cortical surfaces generated by SUFFICIENT display greater continuity compared to those produced by other methods.
